# Supplementary material for: Correctness is not Faithfulness in RAG Attributions
Source: arXiv:2412.18004 source file (2024-12-23)
Supplement: Supplementary file 1 [file appendix.tex]

\section{Appendix}

% \begin{tcolorbox}[
%   tabularx={l|X},
%   title=Summary of Concepts,
%   colbacktitle=blue!40!white,
%   coltitle=black,
%   colframe=blue!25,
%   colback=blue!10!white,
%   fonttitle=\bfseries
% ]
\begin{table}[ht]
\centering
\begin{tabular}{|l|p{11cm}|}
\hline
\textbf{Concept} & \textbf{Description}\\
\hline
Attributed Generation & The process of answer generation with the grounding of the answer through citations to a retrieved set of source documents $A$. \\
&\textit{Example}: Berlin is the \ul{capital} [0] of Germany.\\
\hline
Statement & A text snippet that represents a factual assertion that needs to be grounded in the retrieved documents $A$. Often statements are rather short, even singular words or concepts.\\
&\textit{Example}: \ul{capital}\\
\hline
Claim & The factual assertion underlying the statement that needs to be grounded in the retrieved documents $A$.\\
&\textit{Example}: Berlin is the capital of Germany \\
\hline
Citation & A citation $(s,a)$ connects a statement $s$ to a source document $a\in A$ that supports the stated statement. \\
&\textit{Example}: (capital, 0) \\
\hline
Attribution & The referenced document $a$ or the process of referencing source documents. \\
&\textit{Example}:  0 \\
\hline
Answer Correctness   & The generated statements that form the answer are correct, matching the factual ground truth. This is evaluated most frequently in the open-domain QA and attribution literature.   \\
\hline
Citation Correctness & The cited document $a$ supports the generated statement $s$. Attributions can be incorrect by misrepresenting the content of the attributed documents $A$ or by attributing claims from one document $a$ to another.  \\
\hline
Citation Faithfulness & A citation $(s,a)$ is faithful if the generated statement $s$ is supported by the cited document $a$ (correctness) and the statement $s$ is causally impacted by the cited document $a$.  \\
\hline
Faithfulness & Concept from interpretability and other fields that vaguely descibes how well an explanation reflects the decision process of a model. In the case of attributed generation we differentiate between answer faithfulness (citation correctness) and citation faithfulness \\
\hline
Post-rationalization & A special case of unfaithful behavior where an LLM's parametric memory produces an answer to the question, and the model looks for support in the documents $A$ in some shallow way (e.g., by token-matching).  \\
\hline
\end{tabular}
\caption{Summary of Concepts}
\label{tab:concepts}
\end{table}
% \end{tcolorbox}
